# Supplementary material for: Optimal Control of Wave Energy Converters Using Epsilon-Trig Regularization Method
Source: arXiv:1910.09053 source file (2019-10-20)
Supplement: Supplementary file 1 [file Appendix.tex]

\section*{APPENDIX: TRADITIONAL ANALYTICAL APPROACH}
The WEC problem employing the OCT based traditional approach is described by Eq.~\eqref{eqn:wecan}, where Eq.~\eqref{eqn:wecan1} is the objective functional. Eqs. (\ref{eqn:wecan2})--(\ref{eqn:wecan4}) specify the EOMs for this problem. The Hamiltonian, $H$, is shown in Eq.~\eqref{eqn:wecan5}, which is used to obtain the costate EOMs as shown in Eqs. (\ref{eqn:wecan6})--(\ref{eqn:wecan8}).
\begin{subequations}
\label{eqn:wecan}
\begin{align}
J &= \int_{t_{0}}^{t_{f}}[-ux_{2}]\mathrm{d}t,\label{eqn:wecan1}\\
\dot{x}_{1} &= x_{2},\label{eqn:wecan2}\\
\dot{x}_{2} &= \frac{1}{m} [f\textsubscript{e} - kx_{1} - cx_{2} - u],\label{eqn:wecan3}\\
\dot{x}_{3} &= 1,\label{eqn:wecan4}\\
H &= \lambda_{x_{1}}x_{2} + \dfrac{\lambda_{x_{2}}}{m}[f_{e} - kx_{1} - cx_{2} - u] + \lambda_{x_{3}} - ux_{2},\label{eqn:wecan5}\\
\dot{\lambda}_{x_{1}} &= \dfrac{k\lambda_{x_{2}}}{m},\label{eqn:wecan6}\\
\dot{\lambda}_{x_{2}} &= -\lambda_{x_{1}} + \dfrac{c\lambda_{x_{2}}}{m} + u,\label{eqn:wecan7}\\
\dot{\lambda}_{x_{3}} &= -\frac{\lambda_{x_{2}}\sum_{i=1}^{n}A_{i}\omega_{i}\cos(\omega_{i}x_{3} + \phi_{i})}{m}.\label{eqn:wecan8}
\end{align}
\end{subequations} 
As shown in Eq.~\eqref{eqn:wesing1}, the control, $u$, disappears from the control law, $H_{u} = 0$ since the Hamiltonian, $H$, contains a linear expression of $u$. The first time derivative of the $H_{u}$, $\dot{H}_{u}$, is then calculated as shown in Eq.~\eqref{eqn:wesing2}. The singular control law is obtained if $u$ appears explicitly in the equation, $\ddot{H}_{u} = 0$. Otherwise, further even time derivatives of $H_{u}$ are taken until $u$ appears explicitly in these derivatives. The odd time derivatives of $H_{u}$ serve as additional conditions upon the OCP. For the WEC problem, Eq.~\eqref{eqn:wesing3} specifies the singular control expression for the WEC problem, which uses the condition described in Eq.~\eqref{eqn:wesing2}. Furthermore, the GLCC condition (discussed in Section \ref{sec:bangbang}) for this problem is shown in Eq.~\eqref{eqn:wesing4}, which holds true since $c$ and $m$ are both positive quantities. 
\begin{subequations}
\label{eqn:wesing}
\begin{align}
H_{u} &= \dfrac{-\lambda_{x_{2}}}{m} - x_{2},\label{eqn:wesing1}\\
\dot{H}_{u} &= \dfrac{m(\lambda_{x_{1}} + kx_{1} + cx_{2} - f_{e}) - c\lambda_{x_{2}}}{m^{2}}= 0,\label{eqn:wesing2}\\
u &= \dfrac{1}{2c} [ k\lambda_{x_{2}} + mkx_{2} + 2c(f_{e} - cx_{2} -kx_{1})\notag\\
\ &\ - m\sum_{i=1}^{n}A_{i}\omega_{i}\cos(\omega_{i}x_{3} + \phi_{i})) ],\label{eqn:wesing3}\\
\dfrac{2c}{m} &\geq 0.\label{eqn:wesing4}
\end{align}
\end{subequations}

The traditional approach then requires \textit{a priori} determination of the sequence of control law. This is a lengthy and complicated process that has been omitted from this appendix.
